# Supplementary material for: PEARL: Prompting Large Language Models to Plan and Execute Actions Over Long Documents
Source: arXiv:2305.14564 source file (2023-05-23)
Supplement: Supplementary file 1 [file stats_appendix.tex]

\begin{table*}[]
    \centering
    \footnotesize
    \scalebox{0.75}{
\begin{tabular}{@{}lccccc@{}}
\toprule
            & \multicolumn{1}{c}{\textbf{\compactH}} & \multicolumn{1}{c}{\textbf{\compactM}} & \multicolumn{1}{c}{\compactMNR} & \multicolumn{1}{c}{\compacttwty} & \multicolumn{1}{c}{\compactoneforty} \\ \midrule
\textbf{\# of actions used}   & \multicolumn{1}{c}{81}              & \multicolumn{1}{c}{83}              & \multicolumn{1}{c}{78}       & \multicolumn{1}{c}{41}        & \multicolumn{1}{c}{136}           \\
\textbf{\# of new actions}    & \multicolumn{1}{c}{17}              & \multicolumn{1}{c}{26}              & \multicolumn{1}{c}{18}       & \multicolumn{1}{c}{23}        & \multicolumn{1}{c}{33}            \\
\textbf{\# of steps}          & \multicolumn{1}{c}{3.9}             & \multicolumn{1}{c}{3.9}             & \multicolumn{1}{c}{3.0}      & \multicolumn{1}{c}{3.7}       & \multicolumn{1}{c}{3.1}           \\
\textbf{\# of unique actions} & \multicolumn{1}{c}{3.4}             & \multicolumn{1}{c}{3.4}             & \multicolumn{1}{c}{2.8}      & \multicolumn{1}{c}{3.1}       & \multicolumn{1}{c}{3.0}           \\
\textbf{top-1 action}         & IDENTIFY\_ELEMENT & CONCAT            & CONCAT     & FIND\_ELEMENT                 & CONCAT          \\
\textbf{top-2 action}         & CONCAT            & FIND\_CHARACTER   & FIND\_ELEMENT                & IDENTIFY\_ELEMENT             & FIND\_CHARACTER \\
\textbf{top-3 action}         & FIND\_ELEMENT     & FIND\_ELEMENT     & FIND       & CONCAT      & FIND\_DETAILS   \\
\textbf{top-4 action}         & FIND\_RELATION    & IDENTIFY\_ELEMENT & IDENTIFY\_ELEMENT            & EVALUATE    & FIND\_RELATION  \\
\textbf{top-5 action}         & FIND\_EVENT       & FIND\_EVENT       & FIND\_BEHAVIOR\_REASON       & FIND\_RELATIONSHIP            & FIND\_EVENT     \\ \bottomrule
\end{tabular}
        }
    \caption{compact stats \sscomment{first column, likely put in appendix}}
    \label{tab:compact_stats}
\end{table*}
